# Supplementary material for: Space-time finite element analysis of the advection-diffusion equation using Galerkin/least-square stabilization
Source: arXiv:2307.00822 source file (2024-11-22)
Supplement: Supplementary file 3 [file 6_appendices_stab_no_stab.tex]

\section{Comparison between stabilized and non-stabilized solutions}\label{sec:app:comp-stab-no-stab}
\begin{figure}[!htb]
    \centering
    % Space-time solution with uniform mesh of $128^3$\\
    % \begin{minipage}[t]{.49\textwidth}
    %   \centering
    %   $\kappa = 10^{-2}$
    % \end{minipage}
    % \begin{minipage}[t]{.49\textwidth}
    %   \centering
    %   $\kappa = 10^{-4}$
    % \end{minipage}
    % \\
    \begin{minipage}[t]{.75\textwidth}
      \centering
      \begin{tikzpicture}
      \begin{axis}[
          width=0.99\linewidth, % Scale the plot to \linewidth
          %grid=major, % Display a grid
          %grid style={line width=.1pt, draw=gray!50}, % Set the style
          xlabel=$s$, % Set the labels
          ylabel=$u$,
          legend cell align={left},
          legend style={at={(1,1)},anchor=north east,legend columns=1}, % Put the legend below the plot
          x tick label style={rotate=0,anchor=north} % Display labels sideways
        ]
        \addplot+ [color=blue,dashed,mark=none]
        table[x expr={\thisrow{"arc_length"}},y expr={\thisrow{"u"}},col sep=comma]{results_data/case_2_ad_smoothic_stab_no_stab_comparison/case2_stab_both_lvl5_t0.csv};
        \addplot+ [thick,mark=none]
        table[x expr={\thisrow{"arc_length"}},y expr={\thisrow{"u"}},col sep=comma]{results_data/case_2_ad_smoothic_stab_no_stab_comparison/case2_stab_none_lvl5_t1.csv};
        \addplot+ [thick,mark=none]
        table[x expr={\thisrow{"arc_length"}},y expr={\thisrow{"u"}},col sep=comma]{results_data/case_2_ad_smoothic_stab_no_stab_comparison/case2_stab_space_lvl5_t1.csv};
        \addplot+ [thick,mark=none]
        table[x expr={\thisrow{"arc_length"}},y expr={\thisrow{"u"}},col sep=comma]{results_data/case_2_ad_smoothic_stab_no_stab_comparison/case2_stab_time_lvl5_t1.csv};
        \addplot+ [thick,mark=none]
        table[x expr={\thisrow{"arc_length"}},y expr={\thisrow{"u"}},col sep=comma]{results_data/case_2_ad_smoothic_stab_no_stab_comparison/case2_stab_both_lvl5_t1.csv};
        \legend{
        \small{$t=0$},
        \small{$t=1$, No-stab},
        \small{$t=1$, Stab-spatial},
        \small{$t=1$, Stab-time},
        \small{$t=1$, Stab-both}
        }
      \end{axis}
    \end{tikzpicture}
    \end{minipage}
    \caption{Mesh size: $32^3$}
\end{figure}

\begin{figure}[!htb]
    \centering
    % Space-time solution with uniform mesh of $128^3$\\
    % \begin{minipage}[t]{.49\textwidth}
    %   \centering
    %   $\kappa = 10^{-2}$
    % \end{minipage}
    % \begin{minipage}[t]{.49\textwidth}
    %   \centering
    %   $\kappa = 10^{-4}$
    % \end{minipage}
    % \\
    \begin{minipage}[t]{.49\textwidth}
      \centering
      \begin{tikzpicture}
      \begin{axis}[
          width=0.99\linewidth, % Scale the plot to \linewidth
          %grid=major, % Display a grid
          %grid style={line width=.1pt, draw=gray!50}, % Set the style
          xlabel=$s$, % Set the labels
          ylabel=$u$,
          legend cell align={left},
          legend style={at={(1,1)},anchor=north east,legend columns=1}, % Put the legend below the plot
          x tick label style={rotate=0,anchor=north} % Display labels sideways
        ]
        \addplot+ [color=blue,dashed,mark=none]
        table[x expr={\thisrow{"arc_length"}},y expr={\thisrow{"u"}},col sep=comma]{results_data/case_2_ad_smoothic_stab_no_stab_comparison/case2_stab_both_lvl6_t0.csv};
        \addplot+ [thick,mark=none]
        table[x expr={\thisrow{"arc_length"}},y expr={\thisrow{"u"}},col sep=comma]{results_data/case_2_ad_smoothic_stab_no_stab_comparison/case2_stab_none_lvl6_t1.csv};
        \addplot+ [thick,mark=none]
        table[x expr={\thisrow{"arc_length"}},y expr={\thisrow{"u"}},col sep=comma]{results_data/case_2_ad_smoothic_stab_no_stab_comparison/case2_stab_space_lvl6_t1.csv};
        \addplot+ [thick,mark=none]
        table[x expr={\thisrow{"arc_length"}},y expr={\thisrow{"u"}},col sep=comma]{results_data/case_2_ad_smoothic_stab_no_stab_comparison/case2_stab_time_lvl6_t1.csv};
        \addplot+ [thick,mark=none]
        table[x expr={\thisrow{"arc_length"}},y expr={\thisrow{"u"}},col sep=comma]{results_data/case_2_ad_smoothic_stab_no_stab_comparison/case2_stab_both_lvl6_t1.csv};
        \legend{
        \small{$t=0$},
        \small{$t=1$, No-stab},
        \small{$t=1$, Stab-spatial},
        \small{$t=1$, Stab-time},
        \small{$t=1$, Stab-both}
        }
      \end{axis}
    \end{tikzpicture}
    \end{minipage}
    \caption{Mesh size: $64^3$}
\end{figure}
\clearpage
