# Supplementary material for: Space-time finite element analysis of the advection-diffusion equation using Galerkin/least-square stabilization
Source: arXiv:2307.00822 source file (2024-11-22)
Supplement: Supplementary file 4 [file 6_appendices_stability_higher_order.tex]

%\documentclass[../main.tex]{subfiles}
%\begin{document}

%\end{document}
